# Supplementary material for: InstaNAS: Instance-aware Neural Architecture Search
Source: arXiv:1811.10201 source file (2019-05-23)
Supplement: Supplementary file 1 [file 07-Supplementary.tex]

\begin{appendices}

\section{InstaNAS Overall Algorithm}

    \newcommand{\taskObjective}{\mathop{\mathbb{O}}_{T}}
    \newcommand{\archObjective}{\mathop{\mathbb{O}}_{A}}
    
    \begin{algorithm}[H]
        \caption{\textbf{:} The training phase of InstaNAS consists of three stages: (A) ``pre-train'' the meta-graph, (B) ``jointly train'' both controller and the meta-graph,  and (C) ``fine-tune'' the meta-graph.}
        
        \vspace{0.2em}
        \begin{algorithmic}
            \hspace{-0.8em} \underline{\sc{\textbf{(A) Pre-training}}} \textit{\small \hfill $\vartriangleright$ \underline{7 hours on CIFAR-10}}
        \end{algorithmic}
        \vspace{0.1em}
        \begin{algorithmic}[1]
            \STATE \hspace{0.5em} Profile per-module latency;
            \STATE \hspace{0.5em} Pre-train meta-graph ($G(x;\Theta)$) with $\taskObjective$ only;
        \end{algorithmic}
        
        \vspace{-0.7em}\\\hrulefill \\ [-1.2em]
        \begin{algorithmic}
            \hspace{-0.8em} \underline{\sc{\textbf{(B) \smash{J}oint Training}}} \textit{\small \hfill $\vartriangleright$ \underline{4.5 hours on CIFAR-10}}
        \end{algorithmic}
        \vspace{0.1em}
        \begin{algorithmic}[1]
            \STATE \hspace{0.5em} Initialize $U_t=U_0$ and $L_t=L_0$ for $\archObjective$;
            \STATE \hspace{0.5em} Initialize weight $\phi$ of the controller ($C$);
            \STATE \hspace{0.5em} \textbf{for} {epoch} \textbf{in} \textbf{range} [0,T) \textbf{do}
            \STATE \hspace{1.5em} \textbf{foreach} {iteration} \textbf{do} \textit{\small \hfill $\vartriangleright$ \underline{Train controller}}
            \STATE \hspace{2.5em} $\boldsymbol{p}$ \leftarrow \, $C(x,G;\phi)$;
            \STATE \hspace{2.5em} Sample child architecture weight $\theta_x$ $\sim$ $\boldsymbol{p}$;
            \STATE \hspace{2.5em} Obtain reward $R$ of $m(x;\theta_x)$ from $\taskObjective$ and $\archObjective$;
            \STATE \hspace{2.5em} Update $\phi$ with policy gradient from $R$;
            \STATE \hspace{1.5em} \textbf{end for}
            \STATE \hspace{1.5em} \textbf{foreach} {iteration} \textbf{do} \textit{\small \hfill $\vartriangleright$ \underline{Train meta-graph}}
            \STATE \hspace{2.5em} $\boldsymbol{p}$ \leftarrow \, $C(x,G;\phi)$;
            \STATE \hspace{2.5em} Sample child architecture weight $\theta_x$ $\sim$ $\boldsymbol{p}$;
            \STATE \hspace{2.5em} Obtain loss $L$ of $m(x;\theta_x)$ from $\taskObjective$;
            \STATE \hspace{2.5em} Update $\theta_x$ with gradient from $L$;
            \STATE \hspace{1.5em} \textbf{end for}
            \STATE \hspace{1.5em} Decrease $U_t$ and $L_t$;
            \STATE \hspace{1.5em} Record current ($\phi$, $\Theta$) as ($\phi_{\text{epoch}}$, $\Theta_{\text{epoch}}$);
        \end{algorithmic}
        
        \vspace{-0.7em}\\\hrulefill \\ [-1.2em]
        \begin{algorithmic}
            \hspace{-0.8em} \underline{\sc{\textbf{(C) Fine-Tuning}}} \textit{\small \hfill $\vartriangleright$ \underline{4 hours for each model on CIFAR-10}}
        \end{algorithmic}
        \vspace{0.1em}
        \begin{algorithmic}[1]
            \STATE \hspace{0.5em} Pick N ($\phi_{\text{epoch}}$, $\Theta_{\text{epoch}}$) pairs by preference (different \\
                   \hspace{1.5em} level of trade-offs between $\taskObjective$ and $\archObjective$);
            \STATE \hspace{0.5em} \textbf{foreach} ($\phi_{\text{epoch}}$, $\Theta_{\text{epoch}}$) \textbf{do}
            \STATE \hspace{1.5em} \textbf{while} not converged \textbf{do}
            \STATE \hspace{2.5em} $\boldsymbol{p}$ \leftarrow \, $C(x,G;\phi_{\text{epoch}})$;
            \STATE \hspace{2.5em} $\theta_x \leftarrow \boldsymbol{p}$ (without sampling);
            \STATE \hspace{2.5em} Obtain loss $L$ of $m(x;\theta_x)$ from $\taskObjective$;
            \STATE \hspace{2.5em} Update $\theta_x$ with gradient from $L$;
            \STATE \hspace{1.5em} \textbf{end while}
            \STATE \hspace{0.5em} \textbf{end for}
        \end{algorithmic}
        
    \end{algorithm}
    % \end{minipage}}
    
    \newpage

\section{Numbers of ImageNet Results}
    \vspace{0.5em}
    \begin{table}[h]
        \centering
        % \small
        \vspace{-1em}
        \begin{tabular}{lccr}
            \toprule
            Model & Err. (\%) & Latency \\
            \midrule
            MobileNetV2 $\times$1.0  & 28.2 & 0.257 $\pm$ 0.015  \\
            MobileNetV2 $\times$0.75 & 30.2 & 0.200 $\pm$ 0.012 \\ \hline
            InstaNAS-ImgNet-A & 28.1 & 0.239 $\pm$ 0.014  \\
            InstaNAS-ImgNet-B & 28.9 & \textbf{\underline{0.189}} $\pm$ 0.012 \\
            InstaNAS-ImgNet-C & 30.1 & 0.171 $\pm$ 0.011 \\
            \bottomrule
        \end{tabular}
        \vspace{-0.5em}
        \caption{\small InstaNAS can find model with 14.5\% latency reduction without compromising accuracy on ImageNet. If moderate accuracy drop (0.7\%) is tolerable, InstaNAS-ImgNet-B can further achieve 26.5\% average latency reduction comparing to MobileNetV2 $\times$1.0.}
        \label{table:tiny-imagenet}
        \vspace{-1.5em}
    \end{table}
% \vspace{-0.5em}
\section{Validating the Dynamic Reward} 
% \vspace{-0.5em}
In Figure~\ref{fig.dynamic_vs_static} top panel, we first show the controller policy can steadily follow the dynamic and quadratic latency reward. Then we show the gain of using dynamic reward on the bottom panel. 

% As discussed between lines L428$\sim$L440 of our submission, we consistently observe the static reward is highly unstable and collapses quickly across different sets of hyper-parameters. In Figure~\ref{fig.dynamic_reward}, we conduct an ablation and visualize the convergence to demonstrate this situation.
% \vspace{-1em}
\begin{figure}[h]
\centering
% \minipage{0.4\textwidth}
\includegraphics[width=1\linewidth]{submission/FIG/ICCV_supplementary/converge.png}
% \endminipage\hfill
% \minipage{0.4\textwidth}
\includegraphics[width=1\linewidth]{submission/FIG/ICCV_supplementary/dynamic_vs_static.pdf}
% \endminipage\hfill
\vspace{-1.5em}
\caption{\small\textbf{Top} panel: Training accuracy (top) and latency (bottom) of InstaNAS on CIFAR-10 during \textbf{\textit{search stage}}. The value of dynamic and quadratic latency reward is visualized with colored regions (red color infers higher reward). The result shows that the controller can steadily follow the latency reward and changes over time, until the bound of the latency reward become too strict to satisfy and compensate with accuracy at the same time. We also label the epochs with InstaNAS-C10-\{A-E\}. \textbf{Bottom} panel: The static reward ablation of InstaNAS on CIFAR-10.} 
% We also label the epochs with InstaNAS-C10-\{A-E\}.
% Note that the accuracy requires further fine-tuning to obtain the final accuracy. 
\label{fig.dynamic_vs_static}
\vspace{-0.5em}
\end{figure}

\onecolumn

\section{Search Time and \# Parameters}

    We report the search time and number of parameters of InstaNAS. For search time complexity on CIFAR-10/100 (both 50,000 32x32 images), TinyImageNet (100,000 64x64 images), and ImageNet (1,281,167 224x224 images) datasets, InstaNAS (with 1x TitanXP GPU) takes 7/8/17.5/180 GPU-hours to pre-train the meta-graph and 4.5/5/6/120 GPU-hours to search on target dataset, respectively. The search time complexity does not dramatically increase as the size of the dataset increased. InstaNAS can be considerate as offering a time-space trade-off among architectures. For example, InstaNAS-C10-C has 4.36M parameters, which is 1.90$\times$ of the 2.29M parameters in MobilenetV2\_1.0. However, InstaNAS-C10-C is more accurate and 1.95$\times$ faster than MobilenetV2\_1.0. The search time and number of parameters of InstaNAS also infer that InstaNAS is capable of scaling to a larger and more interesting computer vision problem.

\section{Visualization on Samples Sharing the Same Architecture}
    \vspace{-2em}
    \begin{figure}[h]
      \subfloat[Darker background with clear foreground object.]{
      \includegraphics[width=0.46\linewidth]{submission/FIG/ICCV_supplementary/1.png}} %
      \hfill%
      \subfloat[Lighter background with clear foreground object.]{
      \includegraphics[width=0.495\linewidth]{submission/FIG/ICCV_supplementary/4.png}}\\
      \vspace{-0.85em}
    %   \hfill%
    %   \includegraphics[width=0.495\linewidth]{ICCV_supplementary/FIG/arch_sample_pair/2.png}
    
      \subfloat[Finer-grained textures.]{
      \includegraphics[width=0.495\linewidth]{submission/FIG/ICCV_supplementary/2.png}} %
      \subfloat[Coarser-grained textures.]{
      \includegraphics[width=0.495\linewidth]{submission/FIG/ICCV_supplementary/3.png}}\\
      \vspace{-0.85em}
      
    %   \vspace{1em}
    %   \includegraphics[width=0.495\linewidth]{ICCV_supplementary/FIG/arch_sample_pair/4.png}%
    %   \hfill%
    %   \includegraphics[width=0.495\linewidth]{ICCV_supplementary/FIG/arch_sample_pair/3.png}
      
      \caption{\small We visualize four representative sets of instances and its corresponding architectures. In each sub-figure, the 16 samples on the left-hand side share the same child architecture on the right-hand side. Note that MBConv-A, MBConv-B, MBConv-C, MBConv-D stands for MBConv-3F-3K, MBConv-3F-6K, MBConv-5F-3K, MBConv-5F-6K, respectively.}
      \label{fig:arch-sample-pair}
      \vspace{-1.5em}
    \end{figure}

\section{Implementation Detail}
    For pre-training the meta-graph, we use Stochastic Gradient Descent (SGD) optimizer with naive momentum instead of Nesterov momentum. We set the weight decay as 0.0001 and the momentum as 0.9. The initial learning rate is 0.1, then reduce with cosine annealing through epochs. Each training batch consists of 32 images on a single GPU. Note that larger batch size is preferred if with sufficient memory capacity and computing power.
    
    For the joint training stage, the controller and the meta-graph are trained alternatively for 100 epochs. We set the reward $R_P$ to 30 if the sampled child architecture classifies the corresponding image correctly, otherwise, $R_P$ is set to 0. The upper-bound $U_t$ starts from $U_0 = 2 \overbar{R}_C$, and linearly reduced to half of the MobileNetV2 average latency. The controller is trained with Adam optimizer with learning rate $0.0005$. The meta-graph is fine-tuned with SGD optimizer with cosine annealing learning rate start from $0.01$.

% \vspace{-0.5em}
\section{Visualizing the Distribution of Architectures on TinyImageNet Testing Set}
% \vspace{-0.5em}

\begin{figure*}[h]

  \includegraphics[width=\linewidth]{submission/FIG/Umap/vis_test_im.png}

  \caption{\small Distribution of InstaNAS architectures on TinyImageNet testing set. Each point corresponds to an architecture probability vector $p$. We adopt UMAP to project high-dimensional $p$ into 2D space. More specifically, we first obtain the parametrized transformation function of UMAP on the training set, then use this transformation to project the testing data. For complete and high resolution TinyImageNet training/testing set results, please refer to the following anonymous google drive url: \url{https://goo.gl/yvMRur}.}
  \label{fig:agent-vis-c10}
  \vspace{-1em}
\end{figure*}

\end{appendices}
